# Supplementary material for: Geometric frustration and solid-solid transitions in model 2D tissue
Source: arXiv:1708.07848 ancillary file (2018-03-23)
Supplement: Supplementary file 1 [file SI.pdf]

# Geometric frustration and rigidity transition in 2D tissues

## Supplementary Information

### A CONTINUUM LIMIT OF THE VERTEX MODEL

Our starting point is the discrete Vertex Model energy given in Eq. (1) of the main text and repeated here for convenience

$$E_{\text{VM}} = \sum_{i=1}^N \left[ \frac{1}{2} \kappa_P \left( \frac{P_i - P_0}{P_0} \right)^2 P_0 + \frac{1}{2} \kappa_A \left( \frac{A_i - A_0}{A_0} \right)^2 A_0 \right], \quad (1)$$

where the summation is over all cells,  $\kappa_P$  is the perimeter modulus with dimensions of energy per unit length, and  $\kappa_A$  the area modulus with dimensions of energy per unit area. We consider a lattice of identical hexagonal cells with target area and perimeter  $A_0$  and  $P_0$ . A hexagonal cell is defined by 6 vectors, each positioned at different vertex

$$\tau_n = \cos \frac{2\pi(n-1)}{6} \hat{\mathbf{x}} + \sin \frac{2\pi(n-1)}{6} \hat{\mathbf{y}}, \quad (2)$$

with  $n = 1, \dots, 6$ .

In the continuum limit considered below we assume that each infinitesimal element of the tissue consists of large number of identical cells. To describe cell shape we therefore define a set of unit vectors at each point. More formally, in the continuum limit the unit vectors  $\tau_n$  are defined at every point on the manifold.

In a continuum theory distances are quantified by a metric tensor defined on a differentiable manifold. Denoting by  $\mathbf{g}$  the metric tensor describing a given configuration of the system, the perimeter and area of a cell are then given by

$$P = \sum_{n=1}^6 \sqrt{g_{\mu\nu} \tau_n^\mu \tau_n^\nu}, \quad (3)$$

$$A = \sqrt{\det \mathbf{g}} \Delta S, \quad (4)$$

where  $\mu, \nu \in \{1, 2\}$  and  $\Delta S$  is the area of the polygon spanned by the  $\tau_n$  in units of lattice spacing squared. For the hexagons it is given by

$$\Delta S = \frac{3\sqrt{3}}{2} \quad (5)$$

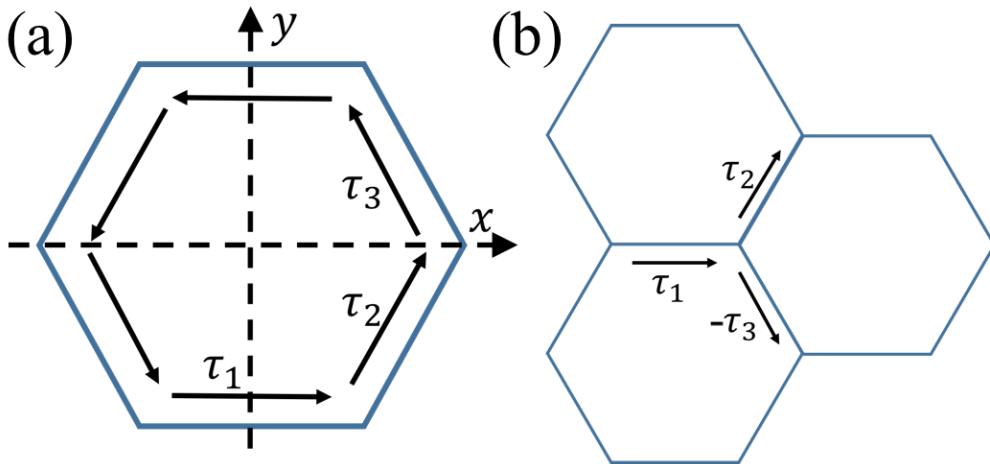

FIG. 1: (a) The tangent vectors  $\tau_n$  of a regular hexagon. (b) Neighboring hexagonal cells sharing the vectors  $\tau_n$ .

in units of the hexagon edge squared. Our goal is to construct a continuum theory that describes the system on length scales large compared to the cell size. An infinitesimal element of the manifold of area  $dS$  will then contain a large number of cells. Assuming a uniform distribution of cells  $\rho_c$ , the number of cells in  $dS$  is then

$$dN = \rho_c dS.$$

The energy of an element of the manifold containing  $dN$  cells can then be written as

$$dE = \left( \frac{1}{2} \kappa_P \left( \frac{\sum_{n=1}^6 \sqrt{g_{\mu\nu} \tau_n^\mu \tau_n^\nu} - P_0}{P_0} \right)^2 P_0 + \frac{1}{2} \kappa_A \left( \frac{\sqrt{\det \mathbf{g}} \Delta S - A_0}{A_0} \right)^2 A_0 \right) \rho_c dS. \quad (6)$$

The total energy is then obtained by integration over the area spanned by the system. In our case, since the tissue is uniform, this corresponds to simply multiplying the energy density by the total area of the tissue.

This is a continuum version of the vertex model which can be studied as a function of its parameters and different external constraints. Equation (6) is, however, not yet written in terms of strains, as needed to obtain new predictions and link with familiar elasticity theory. We now construct the continuum energy in terms of strain as given in Eq. (3) of the main text.

### DERIVATION OF THE CONTINUUM MODEL IN TERMS OF GENERALIZED STRAIN

To express Eq. (6) in terms of strain, it is useful to first briefly recall some basic properties of strains and deformations. Consider a closed curve in the plane of rest length  $l_0$  and stretching modulus  $\kappa$ , with dimensions of energy per unit length. When stretched to a total length  $l$ , the curve stores an elastic energy

$$E_{\text{curve}} = \frac{1}{2} \kappa \left( \frac{l - l_0}{l_0} \right)^2 l_0. \quad (7)$$

If we divide the curve in segments of length  $l_n$ , with  $\sum_n l_n = l$ , each segment has its own rest length  $l_n^0$ , and the elastic energy can also be written as the sum of the contributions from the different elements of the curve, with

$$E_{\text{curve}} = \sum_n \Delta E_n, \quad \Delta E_n = \frac{1}{2} \kappa \left( \frac{l_n - l_n^0}{l_n^0} \right)^2 l_n^0 = \frac{1}{2} \kappa u^2 l_n^0, \quad (8)$$

where we have introduced a strain

$$u = \frac{l - l_0}{l_0} = \frac{l_n - l_n^0}{l_n^0} \quad (9)$$

and made use of the fact that the strain must be uniform along the curve.

Now consider a hexagonal cell of reference perimeter  $P_0$  and actual perimeter  $P$ . Given a hexagonal shaped configuration of the cell, the elastic energy associated with the perimeter of the cell can be written as

$$E_P = \frac{1}{2} \kappa_P \left( \frac{P - P_0}{P_0} \right)^2 P_0 = \sum_{n=1}^6 \frac{1}{2} \kappa_P \left( \frac{l_n - l_n^0}{l_n^0} \right)^2 l_n^0, \quad (10)$$

where  $l_n$  is the actual length of the  $n$ -th edge of the polygon and  $l_n^0$  is the rest length of the edge, satisfying the constraint  $\sum_n l_n^0 = P_0$ , and a uniform strain across the different cell's edges. An alternative to the uniform strain condition is requiring that the rest lengths  $l_n^0$  considered as unknowns and be obtained by minimizing the energy (10) under the constraint  $\sum_n l_n^0 = P_0$ ,

$$E_P = \min_{\{l_n^0\}} \sum_n \frac{1}{2} \kappa_P \left( \frac{l_n - l_n^0}{l_n^0} \right)^2 l_n^0, \quad (11)$$

where the prime on the summation indicates the constraint on the target edge lengths. A direct minimization of Eq. (11) yields the same uniform strain obtained from Eq. (10). This minimization procedure is the analogue of our proposed model in the main text, consisting of a minimization with respect to a set of target metrics.

The energy in (11) is written in terms of lengths rather than target metric. In principle, the rest lengths  $l_n^0$  are functions of the target metric, and  $l_n$  are functions of the actual metric. The minimization operation should therefore be over the space of target metrics. The next calculation, which is based on the classical analysis as presented in Ref. [? ], shows how to rewrite (11) in terms of target and actual metrics.

In Fig. 1(b) we illustrate three neighboring cells sharing three edges and a vertex. The argument presented above suggests that instead of associating an energy with each cell, we can associate an energy per unit perimeter to the shared vertex. The energy is composed of the strains associated with each edge. This observation allows us to follow the standard procedure of constructing a continuum model from a discrete one used for instance in Ref. [? ]. Our derivation follows the same steps, but with some important differences. First, the rest lengths of the different edges are not necessarily unity, but are defined by a target metric. Second, this target metric is in fact the family of all metrics with the same target perimeter. Third, each vertex has three neighbors rather than 6 as in the crystal studied in ref. [? ], labeled here by the index  $k = 1, 2, 3$ . Lastly, we express all quantities in a geometric form in terms of metrics.

The strain on each edge is

$$u^P = \frac{1}{2} (\mathbf{g} - \bar{\mathbf{g}}^P) . \quad (12)$$

One can then associate an energy per unit length with each vertex,

$$\epsilon_{\text{SV}} = \frac{1}{2} \kappa_P \sum_{k=1}^3 (u_{\mu\nu}^P dx_k^\mu dx_k^\nu)^2 . \quad (13)$$

The length element of an edge in differential form is

$$dx_k^\mu = (\bar{\mathbf{g}}^P)^{\mu\nu} \tau_\nu^{(k)} , \quad (14)$$

where  $\tau_\nu^{(k)}$  is the  $k$ 'th tangent vector pointing from the vertex to its neighbor. For the case of hexagonal cellular tissue we have  $\tau^{(k)}$  are given by (2). We therefore find

$$\epsilon_{\text{SV}} = \frac{1}{2} \kappa_P u_{\mu\nu}^P u_{\rho\sigma}^P \left( \sum_{k=1}^3 \sum_{l=1}^3 dx_k^\mu dx_k^\nu dx_l^\rho dx_l^\sigma \right) . \quad (15)$$

By substituting the expressions for  $dx$  and explicit expressions for the tangent vectors  $\tau_\nu$ , we find

$$\left( \sum_{k=1}^3 \sum_{l=1}^3 dx_k^\mu dx_k^\nu dx_l^\rho dx_l^\sigma \right) = \frac{3}{8} [(\bar{\mathbf{g}}^P)^{\mu\nu} (\bar{\mathbf{g}}^P)^{\rho\sigma} + (\bar{\mathbf{g}}^P)^{\mu\rho} (\bar{\mathbf{g}}^P)^{\nu\sigma} + (\bar{\mathbf{g}}^P)^{\mu\sigma} (\bar{\mathbf{g}}^P)^{\nu\rho}] . \quad (16)$$

The energy per unit length of a single vertex can then be written as

$$\epsilon_{\text{SV}} = \frac{1}{2} \mathcal{A}_P^{\mu\nu\rho\sigma} u_{\mu\nu}^P u_{\rho\sigma}^P , \quad (17)$$

with

$$\mathcal{A}_P^{\mu\nu\rho\sigma} = \frac{3}{8} \kappa_P [(\bar{\mathbf{g}}^P)^{\mu\nu} (\bar{\mathbf{g}}^P)^{\rho\sigma} + (\bar{\mathbf{g}}^P)^{\mu\rho} (\bar{\mathbf{g}}^P)^{\nu\sigma} + (\bar{\mathbf{g}}^P)^{\mu\sigma} (\bar{\mathbf{g}}^P)^{\nu\rho}] . \quad (18)$$

To obtain the energy of a uniform tissue associated with perimeter deformations we have to multiply Eq. (17) by  $P_0$ , and by the number of vertices, which is equal to the number of cells. This can be written in general as an integral over the tissue area as

$$E_P = \int \frac{1}{2} \mathcal{A}_P^{\mu\nu\rho\sigma} u_{\mu\nu}^P u_{\rho\sigma}^P P_0 dS_\eta \quad (19)$$

where we have assumed  $\rho_c = 1$  and the cell's area is unity in the fiducial coordinate system.

The above form of the elastic tensor can be compared with the common representation in 2D (see e.g. Ref.[? ])

$$\mathcal{A}^{\alpha\beta\gamma\delta} = \lambda \bar{g}^{\alpha\beta} \bar{g}^{\gamma\delta} + \mu (\bar{g}^{\alpha\gamma} \bar{g}^{\beta\delta} + \bar{g}^{\alpha\delta} \bar{g}^{\beta\gamma}) \quad (20)$$

where  $\lambda$  and  $\mu$  are Lamé constants. Upon absorbing  $P_0$  in (19) into the elastic tensor we find that  $\mathcal{A}_P$  leads to  $\lambda = \mu = 3\kappa_P P_0/8$ .

Next we turn to expressing the single vertex energy associated with area deformations,  $E_A$ , in terms of metrics. The area energy is

$$E_A = \frac{1}{2}\kappa_A \left( \frac{A - A_0}{A_0} \right)^2 A_0 = \frac{1}{2}\kappa_A \frac{(\sqrt{A} - \sqrt{A_0})^2 (\sqrt{A} + \sqrt{A_0})^2}{A_0}.$$

Assuming actual and target metrics  $\mathbf{g}$  and  $\bar{\mathbf{g}}^A$ , the areas for a hexagonal lattice are

$$\begin{aligned} A &= \frac{3\sqrt{3}}{2} \det(\mathbf{g}), \\ A_0 &= \frac{3\sqrt{3}}{2} \det(\bar{\mathbf{g}}^A). \end{aligned} \quad (21)$$

We describe small deviations from the target metric in terms of a strain by writing  $\mathbf{g} \approx \bar{\mathbf{g}}^A + 2u_A$ . Upon expanding to lowest order in powers of  $\epsilon_A$  we obtain a quadratic form in  $u_A$ . Letting  $\frac{1}{2}\mathcal{A}_A^{\mu\nu\rho\sigma}u_{\mu\nu}^A u_{\rho\sigma}^A$  we find

$$\mathcal{A}_A^{\mu\nu\rho\sigma} = \frac{1}{3}\kappa_A A_0 (2(\bar{\mathbf{g}}^A)^{\mu\nu}(\bar{\mathbf{g}}^A)^{\rho\sigma} + (\bar{\mathbf{g}}^A)^{\mu\rho}(\bar{\mathbf{g}}^A)^{\nu\sigma} + (\bar{\mathbf{g}}^A)^{\mu\sigma}(\bar{\mathbf{g}}^A)^{\nu\rho}). \quad (22)$$

We stress that other cellular lattices will modify the numerical factors in the expressions for the perimeters  $P, P_0$  and the areas  $A, A_0$ , and therefore the values of the Lamé coefficients. The details of the calculation for a hexagonal lattice are presented in an attached *Mathematica* notebook.

As before, the target area by itself does not determine a target metric. Therefore, like above, here  $\bar{\mathbf{g}}^A$  stands for the equivalence class of all target metrics describing the same target area  $A_0$ . The energy associated with area deformations is then

$$E_A = \int \frac{1}{2}\mathcal{A}_A^{\mu\nu\rho\sigma}u_{\mu\nu}^A u_{\rho\sigma}^A dS_\eta. \quad (23)$$

## EXPLICIT REPRESENTATIONS OF $G_A$ AND $G_P$ FOR A HEXAGONAL UNIT CELL

Let us consider a regular hexagon whose target area  $A_0$  is described by the target metric

$$\bar{\mathbf{g}}^A = \alpha_A \begin{pmatrix} 1 & 0 \\ 0 & 1 \end{pmatrix}, \quad (24)$$

with  $A_0 = \sqrt{\det[\bar{\mathbf{g}}^A]} \int_S d^2\mathbf{x} = \alpha_A \Delta S$ . The integration  $\int_S$  is over the cell region, and quantify its area in the fiducial coordinate system. As already mentioned, in our case this is the area spanned by the tangent vectors  $\tau_i$ :  $\Delta S = 3\sqrt{3}/2$ . The hexagon can, however, be stretched along the  $y$  direction and compressed in the  $x$  direction while preserving its area. Hexagons of area  $A_0$  are therefore described by a family of target metrics, given by

$$\bar{\mathbf{g}}^A = \alpha_A \begin{pmatrix} \epsilon_A & 0 \\ 0 & 1/\epsilon_A \end{pmatrix}, \quad (25)$$

and parametrized by  $\epsilon_A$ . Additional area-preserving shapes can be obtained by shearing the hexagon, corresponding to off-diagonal components of the target metric. In this work, for simplicity, we do not consider such deformations.

Similarly, let us consider a hexagon of reference perimeter  $P_0 = 6\alpha_P$  described by the target metric

$$\bar{\mathbf{g}}^P = \alpha_P^2 \begin{pmatrix} 1 & 0 \\ 0 & 1 \end{pmatrix}. \quad (26)$$

In particular, the tangent vectors for a regular hexagon of perimeter 6 in a fiducial coordinate system are given in Eq. (2) and shown in Fig. 1. The perimeter  $P_0$  is then given by

$$P_0 = \sum_{n=1}^6 \sqrt{g_{\mu\nu}^P \tau_n^\mu \tau_n^\nu} = 6\alpha_P. \quad (27)$$

We now stretch the hexagon along the  $y$  direction and compress it in the  $x$  direction. The perimeter of the deformed hexagon is described by the metric

$$\bar{\mathbf{g}}^P = \alpha_P^2 \begin{pmatrix} \epsilon_P^2 & 0 \\ 0 & \epsilon_x \end{pmatrix}. \quad (28)$$

We determine  $\epsilon_x$  by requiring that this transformation preserve the perimeter. The perimeter with the deformed target metric is

$$P'_0 = 2\sqrt{g^P_{\mu\nu}\tau_1^\mu\tau_1^\nu} + 2\sqrt{g^P_{\mu\nu}\tau_2^\mu\tau_2^\nu} + 2\sqrt{g^P_{\mu\nu}\tau_3^\mu\tau_3^\nu} = 2\alpha_P \left( \epsilon_P + \sqrt{\frac{\epsilon_P^2}{4} + \frac{3\epsilon_x}{4}} + \sqrt{\frac{\epsilon_P^2}{4} + \frac{3\epsilon_x}{4}} \right) \quad (29)$$

Requiring  $P'_0 = 6\alpha_P$ , we find  $\epsilon_x = 3 - 2\epsilon_P$ . The family of perimeter preserving target metrics that correspond to stretching/compressing along  $x$  and  $y$  directions is then given by

$$\bar{\mathbf{g}}^P = \alpha_P^2 \begin{pmatrix} \epsilon_P^2 & 0 \\ 0 & 3 - 2\epsilon_P \end{pmatrix}. \quad (30)$$

### THE TARGET CELL SHAPE INDEX

The perimeter of a hexagon with the above metric  $\bar{\mathbf{g}}^P$  is independent of  $\epsilon_P$  and is  $P_0 = 6\alpha_P$  in units of the lattice constant. The area of a hexagon with the reference metric  $\bar{\mathbf{g}}_A$  is independent of  $\epsilon_A$  and is  $A_0 = \frac{3\sqrt{3}}{2}\alpha_A$ . The shape parameter is then

$$s_0 = \frac{P_0}{\sqrt{A_0}} = \frac{6\alpha_P}{\sqrt{\frac{3\sqrt{3}}{2}\alpha_A}}. \quad (31)$$

A perfect hexagon corresponds to  $\alpha_P = \alpha_A = 1$  and therefore  $s_0 = \sqrt{8\sqrt{3}} = 3.72242$ . It is clear that for small strains our model fits the exact one pretty well. As strains increase, or alternatively, as incompatibility increases, our model becomes less accurate. Still, the relatively good agreement between the models justifies the study of our model and its predictions.

### EXPLICIT FORM OF THE ENERGY AND RESPONSE TO EXTERNAL STRAIN

To obtain an explicit expression for the energy of a cellular tissue we insert the representations of the reference metrics  $\bar{\mathbf{g}}^P$  and  $\bar{\mathbf{g}}^A$  in terms of  $\epsilon_P$  and  $\epsilon_A$  in equation 3 of the main text. For simplicity we consider the case of uniaxial deformations in the  $x$  direction, when the actual metric remains diagonal. All components of the metric tensor are a priori finite for general deformations. The energy is measured in units of  $\kappa_P P_0$  and the metric components are measured in units of  $\alpha_A$ . Then, the energy functional is fully determined in terms of two dimensionless parameters:  $\xi = \alpha_A/\alpha_P^2 = \frac{\sqrt{3}}{24}s_0^2$  quantifying the amount of incompatibility, and  $\zeta = \frac{A_0\kappa_A}{P_0\kappa_P}$ , measuring the ease of perimeter deformations ( $1 \ll \zeta$ ) vs area deformations ( $\zeta \ll 1$ ). The total energy is then given by

$$E(\mathbf{g}) / (\kappa_P P_0) = \min_{\epsilon_A, \epsilon_P} E_P + E_A \quad (32)$$

with

$$E_P(\mathbf{g}) = \frac{3(\xi^2(3g_{11}^2(3-2\epsilon_P)^2 + 2g_{11}g_{22}(3-2\epsilon_P)\epsilon_P^2 + 3g_{22}^2\epsilon_P^4) + 8\xi(2\epsilon_P-3)\epsilon_P^2(g_{11}(3-2\epsilon_P) + g_{22}\epsilon_P^2) + 8(3-2\epsilon_P)^2\epsilon_P^4)}{16(3-2\epsilon_P)^2\epsilon_P^4} \quad (33)$$

and

$$E_A(\mathbf{g}) = \frac{2\zeta(g_{11}^2 + g_{11}\epsilon_A(g_{22}\epsilon_A - 3) + \epsilon_A^2(g_{22}\epsilon_A(g_{22}\epsilon_A - 3) + 3))}{3\epsilon_A^2} \quad (34)$$

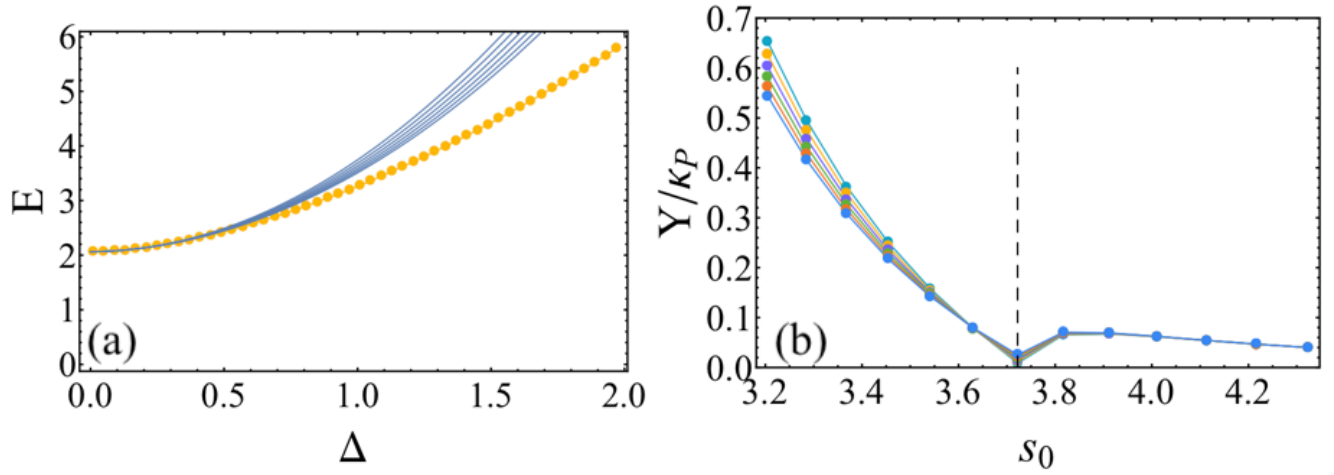

FIG. 2: (a) Energy-Strain curve of an incompatible tissue (yellow dots) and fits to a parabola (blue lines). The different blue curves correspond to different windows of strain used in the fitting procedure, from 0-0.05% to 0-0.5%. (b) The corresponding effective Young's modulus extracted from the fitted parabolas as a function of the shape parameter. Each curve corresponds to a different strain range used in the fit.

We study the model as function of the two dimensionless parameter. In the main text we represent the results in terms of the shape index parameter  $s_0$  rather than  $\xi$ . Given  $s_0$ , and  $\zeta$ , we find the ground state by minimizing  $E$  with respect to  $a_{11}, a_{22}, \epsilon_A, \epsilon_P$ .

To measure the response of our tissue model to external strain we first fix  $a_{11}$  and minimize the energy with respect to  $a_{22}, \epsilon_A, \epsilon_P$ .

We also study the elastic response to external strain  $a_{11}$  while transverse strain is fixed through  $a_{22}$ , by minimizing only with respect to  $\epsilon_A$  and  $\epsilon_P$ .

## NON-UNIFORM CELLULAR TISSUE

In the attached Mathematica notebook we present an example of a cellular tissue with non-uniform shape parameter confined to cylindrical geometry.

## YOUNG'S MODULUS - THE FITTING PROCEDURE

The effective Young's modulus shown in Fig. 3 of the main text is calculated by fitting the energy-strain curves to a parabola. Since in the incompatible regime such curves are in general not quadratic in the strain, as shown in Fig. 2(b), it is not obvious what range of strain should be used beyond the origin in the fitting procedure. In Fig. 2(b) we show the Young's modulus calculated by fitting the energy using different choices of strain ranges (0-0.05% to 0-0.5%). The data shown in the main text are obtained by fitting in a strain range of 0-0.5%. The interested reader can easily modify this choice in the Mathematica notebook attached to our manuscript to verify the dependence of the Young modulus on the fitting range.

## EXTRA DATA

Here, for the convenience of the interested reader, we show two additional plots related with the data shown in the main text. In Fig. 3 we plot the force-extension curve derived from Fig.2(a) in the main text. In Fig. 4 we plot the force-extension curves for incompatible tissue on a log-log scale, highlighting the inherent nonlinear response.

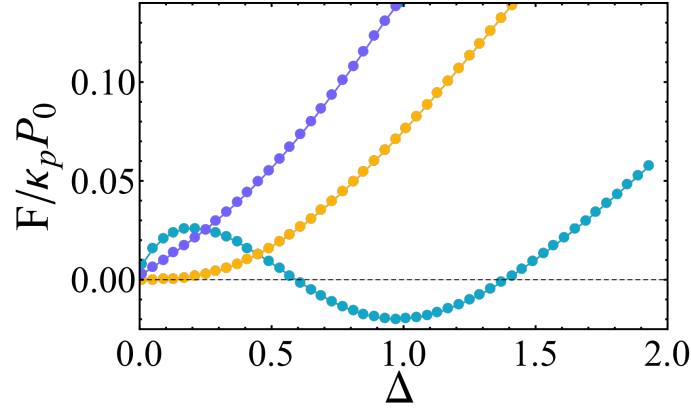

FIG. 3: Force  $F = -\frac{\partial E}{\partial \Delta}$  vs. strain for  $\zeta = 1$  and  $s_0 = 3.874$  (compatible, light-blue),  $s_0 = 3.722$  (critically compatible, yellow), and  $s_0 = 3.577$  (incompatible, dark-blue). The negative force obtained for the compatible tissue reflects the instability associated with the double-well in the energy.

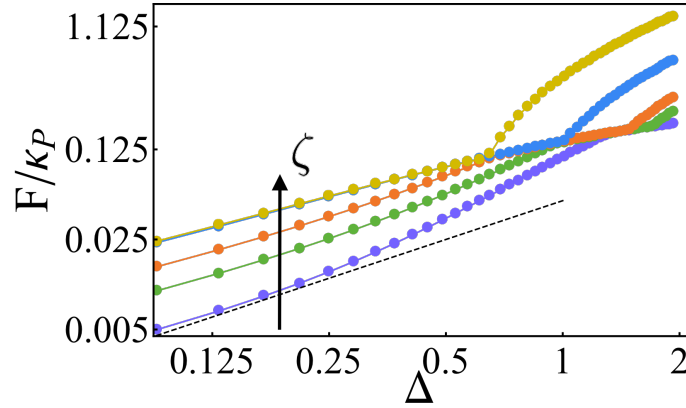

FIG. 4: Force-extension curves for incompatible tissue for  $s_0 = 3.577, 3.438, 3.303, 2.932, 2.5$ , showing sharp strain stiffening at large strains. The black dashed line has slope one and is shown to highlight the deviation from linear behavior.

### TRANSVERSE-STRAIN STIFFENING

In Fig. 5 we plot the effective Young's modulus in response to strain along the  $x$  direction as function of the fixed transverse strain  $\Delta_{yy}$ . Each curve correspond to a different value of the shape index: light-blue is compatible, yellow is critically compatible, and purple is incompatible. In contrast with linear elasticity, here we find that the effective Young's modulus show a rigidity transition as the transverse strain is increased, demonstrating the inherent nonlinearity of our model.

### A SINGLE REFERENCE METRIC FORMULATION

In our model the energy associated with an elastic tissue whose configuration is  $\mathbf{g}$  is given by

$$E_{\text{tissue}}(\mathbf{g}) = \min_{G_A} \min_{G_P} \int_{\Omega} \frac{1}{2} \mathcal{A}_A^{\alpha\beta\gamma\delta} u_{\alpha\beta}^A u_{\gamma\delta}^A dS_{\mathbf{g}^A} + \int_{\Omega} \frac{1}{2} \mathcal{A}_P^{\alpha\beta\gamma\delta} u_{\alpha\beta}^P u_{\gamma\delta}^P dS_{\mathbf{g}^P}, \quad (35)$$

Defining

$$\begin{aligned} \bar{\mathbf{g}}_{\alpha\beta}^0 &= \bar{\mathcal{A}}_{\alpha\beta\gamma\delta}^{-1} \left( \mathcal{A}_P^{\gamma\delta\mu\nu} \sqrt{|\bar{\mathbf{g}}^P|} \bar{\mathbf{g}}_{\mu\nu}^P + \mathcal{A}_A^{\gamma\delta\mu\nu} \sqrt{|\bar{\mathbf{g}}^A|} \bar{\mathbf{g}}_{\mu\nu}^A \right) \\ \bar{\mathcal{A}} &= \mathcal{A}_P \sqrt{|\bar{\mathbf{g}}^P|} + \mathcal{A}_A \sqrt{|\bar{\mathbf{g}}^A|} \end{aligned} \quad (36)$$

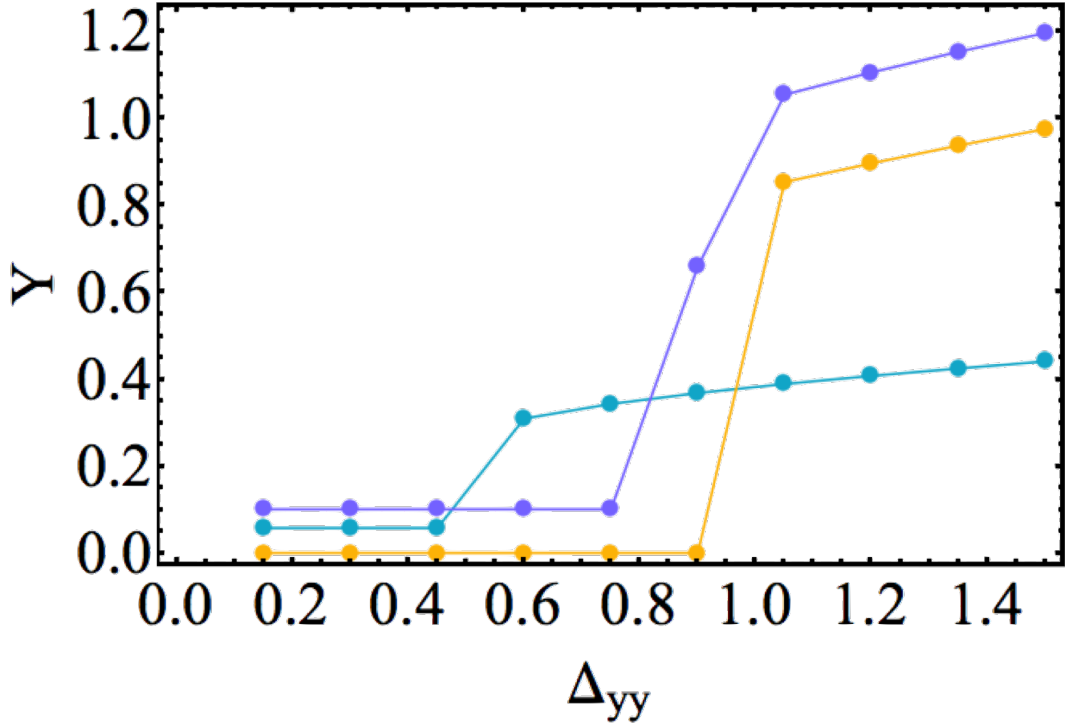

FIG. 5: The effective Young's modulus in response to strain along the  $x$  direction, as function of a fixed transverse strain, for  $s_0 = 4.031$  (light-blue),  $s_0 = 3.722$  (yellow), and  $s_0 = 3.437$  (purple).

with  $\mathcal{A}_0 = \bar{\mathcal{A}}/\sqrt{|\bar{\mathbf{g}}^0|}$ ,  $u^0 = \frac{1}{2}(\mathbf{g} - \bar{\mathbf{g}}^0)$ , and

$$\|\bar{\mathbf{g}}\|^2 = \mathcal{A}_0^{\alpha\beta\gamma\delta} \bar{\mathbf{g}}_{\alpha\beta} \bar{\mathbf{g}}_{\gamma\delta} \sqrt{|\bar{\mathbf{g}}|}. \quad (37)$$

we complete the square and get

$$E_{\text{Eff}} = \min_{G_A, G_P} \frac{1}{2} \int_{\Omega} \mathcal{A}_0^{\alpha\beta\gamma\delta} u_{\alpha\beta}^0 u_{\gamma\delta}^0 \sqrt{|\bar{\mathbf{g}}^0|} d^2\mathbf{x} + E_{\text{res}}, \quad (38)$$

with the residual energy  $E_{\text{res}}(\bar{\mathbf{g}}^0, \bar{\mathbf{g}}^P, \bar{\mathbf{g}}^A)$  given by

$$E_{\text{res}} = \int_{\Omega} \left( \|\bar{\mathbf{g}}^P\|^2 + \|\bar{\mathbf{g}}^A\|^2 - \|\bar{\mathbf{g}}^0\|^2 \right) d^2\mathbf{x}. \quad (39)$$

## ANALOGY WITH MECHANICS OF AMORPHOUS SOLIDS

In the incompatible case, in the absence of external loads, the equilibrium configuration is given by the actual metric and reference metrics that minimize  $E_{\text{tissue}}$ , denoted in the main text by  $\mathbf{g}_*$ ,  $\bar{\mathbf{g}}_*^A$ ,  $\bar{\mathbf{g}}_*^P$ . As discussed in the main paper, when the tissue is strained the reference geometry may deform within the sets  $G_A$  and  $G_P$ . We denote such deviations of  $\bar{\mathbf{g}}^A$  and  $\bar{\mathbf{g}}^P$  from the values  $\bar{\mathbf{g}}_*^A$  and  $\bar{\mathbf{g}}_*^P$  by  $\delta\bar{\mathbf{g}}^A$ , and  $\delta\bar{\mathbf{g}}^P$ . These quantities are clearly functions of the external constraints. Variations of the metrics within the families  $G_A$  and  $G_P$  preserve area and perimeter and are therefore interpreted as zero modes in the compatible tissue. In the incompatible case, however, a finite energetic cost is associated with such deformations. Letting  $\delta\epsilon = \{\delta\bar{\mathbf{g}}^A, \delta\bar{\mathbf{g}}^P\}$  and expanding the energy in terms of these variations one finds

$$E_{\text{Eff}} \approx \frac{1}{2} \int_{\Omega} \left( \mathcal{A}_0^{\alpha\beta\gamma\delta} u_{\alpha\beta}^0 u_{\gamma\delta}^0 + \mathcal{E}_2^{\mu\nu} \delta\epsilon_{\mu} \delta\epsilon_{\nu} \right) dS_{\bar{\mathbf{g}}^0}. \quad (40)$$

In the compatible case  $\mathcal{E}_2^{\mu\nu}$  vanishes identically. In contrast, in the incompatible case where a zero energy configuration does not exist,  $\mathcal{E}_2^{\mu\nu}$  is positive definite, and therefore acts as an energetic cost associated with any finite  $\delta\epsilon$ . Since  $\delta\epsilon$  modifies  $\bar{\mathbf{g}}_0$ , it modifies the reference geometry and it is therefore interpreted as an anelastic deformation.

As explained in the main text, (40) draws an analogy with the mechanics of amorphous solids, where anelastic deformations are associated with an energetic cost due to self-interaction energy which is quadratic in the strain that describes such deformations. This analogy may be used to port knowledge from the well established field of mechanics of amorphous solids to that of cellular tissues and vertex model.

- 
- S. H. Seung and D. R. Nelson, Phys. Rev. A **38**, 1005 (1988).
  - E. Efrati, E. Sharon, and R. Kupferman, JMPS **57**, 762 (2009).
